# Supplementary material for: Perception of AI-Generated Music -- The Role of Composer Identity, Personality Traits, Music Preferences, and Perceived Humanness
Source: arXiv:2512.02785 ancillary file (2025-12-02)
Supplement: Supplementary file 1 [file Supplements.pdf]

# Supplements

## A. Stimuli Generation

### S1: Prompt List

| Music Genre | Subgenre | GEMS-Item | Prompt (Suno v. 3.5, instrumental mode) | Prompt (Stable Audio, v. 2.0) |
|---|---|---|---|---|
| Electro | Trance | Joyful Activation | a joyful, bouncy, animated trance song | Trance, joyful, bouncy, animated, instrumental |
| Electro | Trance | Power | a strong, energetic, triumphant trance song | Trance, strong, energetic, triumphant, instrumental |
| Funk/Soul | Disco | Joyful Activation | a joyful, bouncy, animated disco song | Disco, joyful, bouncy, animated, instrumental |
| Funk/Soul | Disco | Power | a strong, energetic, triumphant disco song | Disco, strong, energetic, triumphant, instrumental |
| Funk/Soul | Funk | Joyful Activation | a joyful, bouncy, animated funk song | Funk, joyful, bouncy, animated, instrumental |
| Funk/Soul | Funk | Power | a strong, energetic, triumphant funk song | Funk, strong, energetic, triumphant, instrumental |
| Pop | Pop-Punk | Joyful Activation | a joyful, bouncy, animated pop-punk song | Pop-Punk, joyful, bouncy, animated, instrumental |
| Pop | Pop-Punk | Power | a strong, energetic, triumphant pop-punk song | Pop-Punk, strong, energetic, triumphant, instrumental |
| Pop | Europop | Joyful Activation | a joyful, bouncy, animated europop song | Europop, joyful, bouncy, animated, instrumental |
| Pop | Europop | Power | a strong, energetic, triumphant europop song | Europop, strong, energetic, triumphant, instrumental |
| Electro | Downtempo | Tenderness | a romantic, tender, affectionate downtempo song | Downtempo, romantic, tender, affectionate, instrumental |
| Electro | Downtempo | Peacefulness | a relaxed, calm, soothed downtempo song | Downtempo, relaxed, calm, soothed, instrumental |
| Electro | Downtempo | Nostalgia | a nostalgic, sentimental, dreamy downtempo song | Downtempo, nostalgic, sentimental, dreamy, instrumental |
| Funk/Soul | Soul | Tenderness | a romantic, tender, affectionate soul song | Soul, romantic, tender, affectionate, instrumental |
| Funk/Soul | Soul | Peacefulness | a relaxed, calm, soothed soul song | Soul, relaxed, calm, soothed, instrumental |
| Funk/Soul | Soul | Nostalgia | a nostalgic, sentimental, dreamy soul song | Soul, nostalgic, sentimental, dreamy, instrumental |
| Jazz | Swing | Tenderness | a romantic, tender, affectionate swing song | Swing, romantic, tender, affectionate, instrumental |
| Jazz | Swing | Peacefulness | a relaxed, calm, soothed swing song | Swing, relaxed, calm, soothed, instrumental |
| Jazz | Swing | Nostalgia | a nostalgic, sentimental, dreamy swing song | Swing, nostalgic, sentimental, dreamy, instrumental |
| Jazz | Bossa-Nova | Tenderness | a romantic, tender, affectionate bossa-nova song | Bossa-Nova, romantic, tender, affectionate, instrumental |
| Jazz | Bossa-Nova | Peacefulness | a relaxed, calm, soothed bossa-nova song | Bossa-Nova, relaxed, calm, soothed, instrumental |
| Jazz | Bossa-Nova | Nostalgia | a nostalgic, sentimental, dreamy bossa-nova song | Bossa-Nova, nostalgic, sentimental, dreamy, instrumental |
| Jazz | Smooth Jazz | Tenderness | a romantic, tender, affectionate smooth-jazz song | Smooth-Jazz, romantic, tender, affectionate, instrumental |

| | | | | |
|---|---|---|---|---|
| Jazz | Smooth Jazz | Peacefulness | a relaxed, calm, soothed smooth-jazz song | Smooth-Jazz, relaxed, calm, soothed, instrumental |
| Jazz | Smooth Jazz | Nostalgia | a nostalgic, sentimental, dreamy smooth-jazz song | Smooth-Jazz, nostalgic, sentimental, dreamy, instrumental |
| Pop | Indie-Pop | Tenderness | a romantic, tender, affectionate indie-pop song | Indie-Pop, romantic, tender, affectionate, instrumental |
| Pop | Indie-Pop | Peacefulness | a relaxed, calm, soothed indie-pop song | Indie-Pop, relaxed, calm, soothed, instrumental |
| Pop | Indie-Pop | Nostalgia | a nostalgic, sentimental, dreamy indie-pop song | Indie-Pop, nostalgic, sentimental, dreamy, instrumental |
| Rock | Ballad | Tenderness | a romantic, tender, affectionate rock ballad | Rock ballad, romantic, tender, affectionate, instrumental |
| Rock | Ballad | Peacefulness | a relaxed, calm, soothed rock ballad | Rock ballad, relaxed, calm, soothed, instrumental |
| Rock | Ballad | Nostalgia | a nostalgic, sentimental, dreamy rock ballad | Rock ballad, nostalgic, sentimental, dreamy, instrumental |
| Rock | Soft-Rock | Tenderness | a romantic, tender, affectionate soft-rock song | Soft-Rock, romantic, tender, affectionate, instrumental |
| Rock | Soft-Rock | Peacefulness | a relaxed, calm, soothed soft-rock song | Soft-Rock, relaxed, calm, soothed, instrumental |
| Rock | Soft-Rock | Nostalgia | a nostalgic, sentimental, dreamy soft-rock song | Soft-Rock, nostalgic, sentimental, dreamy, instrumental |
| Electro | Dubstep | Tension | a tense, irritating, agitating dubstep song | Dubstep, tense, irritating, agitating, instrumental |
| Electro | Dubstep | Power | a strong, energetic, triumphant dubstep song | Dubstep, strong, energetic, triumphant, instrumental |
| Rock | Doom-Metal | Tension | a tense, irritating, agitating doom-metal song | Doom-Metal, tense, irritating, agitating, instrumental |
| Rock | Doom-Metal | Power | a strong, energetic, triumphant doom-metal song | Doom-Metal, strong, energetic, triumphant, instrumental |

**Detailed description for prompt generation and editing**

To account for the properties of each tool, the following approach was used: For Suno, the standard instrumental mode was used, with each prompt returning two audio outputs. To avoid bias in stimulus selection, one of the two outputs was randomly chosen for inclusion in the study. Since the output lengths of the Suno-generated songs are arbitrary and vary considerably, the songs were manually cut to 45-60 seconds versions to be comparable to previous research. Editing was based on musical considerations, such as phrasing and structural cues (e.g., completing a chorus or musical idea), to ensure that excerpts felt coherent and musically resolved. All edits began at the start of the track and used fade-out transitions to create natural endings. For Stable Audio, the word “instrumental” was added to each prompt to prevent the inclusion of vocals, as the tool does not offer a separate instrumental mode. The target duration for each generation was set to 60 seconds. Because the duration is specified in advance, the tool automatically creates a fade-out, aiming to shape a musically coherent segment that ends smoothly within the time constraint.

**Link to Audio-Files:**

## B. Additional Analyses of Individual Differences

**Table S2. Correlations of personality and music-related variables with liking and emotional intensity**

(Pearson correlations, two-tailed. Significant effects in bold.)

| | Liking | | Emotional Intensity | |
|---|---|---|---|---|
| **Predictor** | **r** | **p** | **r** | **p** |
| **Attitudes toward AI (ATTARI)** | | | | |
| – Total | 0.37 | <.001 | 0.31 | <.001 |
| – Affective | 0.32 | <.001 | 0.25 | <.001 |
| – Cognitive | 0.31 | <.001 | 0.28 | <.001 |
| **– Behavioral** | 0.40 | <.001 | 0.34 | <.001 |
| **Music Usage (UMI)** | | | | |
| – Emotional | 0.27 | <.001 | 0.27 | <.001 |
| – Cognitive | 0.23 | .002 | 0.34 | <.001 |
| – Background | 0.15 | .043 | 0.20 | .006 |
| **Genre Preferences (STOMP)** | | | | |
| – Reflective/Complex | 0.24 | .001 | 0.26 | <.001 |
| – Intense/Rebellious | 0.06 | .438 | -0.02 | .791 |
| – Upbeat/Conventional | 0.29 | <.001 | 0.25 | .001 |
| – Energetic/Rhythmic | 0.14 | .057 | 0.18 | .016 |
| **Big Five Personality** | | | | |
| – Openness | -0.05 | .469 | -0.08 | .276 |
| – Conscientiousness | 0.28 | <.001 | 0.24 | <.001 |
| – Extraversion | 0.10 | .180 | 0.12 | .099 |
| – Agreeableness | 0.23 | .002 | 0.12 | .100 |
| – Neuroticism | -0.36 | <.001 | -0.29 | <.001 |
| **Music Mindedness (MMQ)** | | | | |
| – Cognitive | 0.22 | .004 | 0.33 | <.001 |
| – Affective | 0.21 | .005 | 0.28 | <.001 |
| **Demographics** | | | | |
| – Age | 0.11 | .150 | -0.06 | .451 |
| – Gender | - 0.06 | .422 | 0.10 | .192 |
| – Consider yourself musician | 0.09 | .229 | 0.24 | .002 |
| – Weekly listening hours | 0.12 | .109 | 0.16 | .034 |

**Table S3. Effects of ATTARI subscales on liking and emotional intensity (mixed-effects models)**

| | Liking | | Emotional Intensity | |
|---|---|---|---|---|
| **Predictor** | **β** | **p** | **β** | **p** |
| Affective | -0.01 | .93 | -0.09 | .43 |
| Cognitive | -0.02 | .83 | 0.05 | .61 |
| Behavioral | 0.14 | .031 | 0.21 | .028 |

**Table S4. Moderation analyses of experimental condition × AI attitudes (mixed-effects models)**

| | Liking | | Emotional Intensity | |
|---|---|---|---|---|
| **Interaction term** | **ß** | **p** | **β** | **p** |
| **ATTARI Total** | | | | |
| – Human × ATTARI | -0.13 | .325 | -2.15 | .450 |
| – No-info × ATTARI | -0.05 | .710 | 0.00 | .999 |
| **ATTARI Behavioral** | | | | |
| – Human × ATTARI BEH | -0.02 | .877 | -0.87 | .715 |
| – No-info × ATTARI BEH | -0.01 | .926 | 0.62 | .796 |

## C. Thematic Analysis for Listener evaluation criteria for AI-Generated Music

Phrasing of open-ended question: "“What is your personal opinion on AI-generated music? Please briefly describe your thoughts on it and explain which aspects you find particularly appealing or potentially critical. Please report your own (human) thoughts and do not use AI to answer this question ;)”

**Table S5. Codebook for Thematic Analysis of open-ended questions**

| Main Theme | Subcode | Definition | Illustrative Quote |
|---|---|---|---|
| Music Quality | Creativity / (Lack of) Originality | Song-level judgements about novelty, originality, or repetitiveness. | „that AI generates music that always sound pretty similar“ (Original: „dass die KI Musik generiert, die immer ziemlich ähnlich klingt.“), ID84 |
| | Technical musical quality | Judgements of production and sound engineering, digital artifacts, and whether the music is technically correct or flawed. | “Sometimes it was rather crooked, so I thought it was generated” (Original: “manchmal war es eher schief da dachte ich schon das es generiert ist”), ID79 |
| | Musical structure | Arrangement (build-up, transitions, coherence, endings). | "“ With longer playing times, it becomes clearly audible that there is no build-up of tension or drama here.” (Original: “bei längerer Laufzeit deutlich hörbar, dass hier keinerlei Spannungsaufbau oder Dramaturgie vorhanden ist“, ID68 |
| | Musical features | Description of musical elements (melody, harmony, rhythm). | “the drums beats and the tune seem repetitive”, ID444 |
| Importance of Humanness | (Lack of) Soul / Human Touch | Presence/absence of human expressiveness, feel, or soul. | “It sounds polished, but lacks the soul and story behind it.”, ID912 |
| | Authenticity | Concerns about whether AI-generated music can be considered authentic | “I love the beats but I feel like they not authentic”, ID421 |

| | | | |
|---|---|---|---|
| | Personality / History of an Artist | Evaluations emphasizing the importance of an artist's personal story, history, and emotions behind music | "Nevertheless, I prefer to listen to music composed by real people; I think there is much more history, thought, and emotion behind it. (Original: „Trotzdem höre ich lieber Musik die von echten Menschen komponiert wurde, ich finde da steckt viel mehr Geschichte, Gedanken und Emotionen dahinter."), ID404 |
| | Perceived (In)distinguishability | Claims AI and human music sound similar/indistinguishable, or if is origin irrelevant. | "If it sounds good then I don't mind if it was artificially generated.", ID926 |
| Emotional aspects | Negative emotions | Expressions of annoyance, unease, fear elicited by the excerpt | "It is the part of AI that scares me." ID446 |
| | Positive emotions | Expressions of enjoyment, fun, relaxation, uplift, nostalgia | "I found AI music relaxing and very entertaining." ID216 |
| | Emotional capabilities / depth | Judgements whether and how strong AI can convey emotion | "it may lack emotional depth" ID208 |
| Attitudes toward AI | Normative statements about AI | Principled positions about what art should/should not be | I think art, in this case music, should be produced by humans (Original: "Ich finde Kunst, in dem Falle Musik, sollte von Menschen produziert warden"), ID45 |
| | General neglection of AI music | Blanket rejection/aversion toward AI music as a category | "I think AI generated music is nonsense. Why do we need it?" ID952 |
| | General statements on AI | Broad non-musical appraisals of AI | "AI has been more advantageous to the world than it has been an instrument of destruction" ID453 |
| Ethical considerations | Economic implications on artists | Considerations about negative impacts on value of artistic work and market | "It also takes away jobs from real musicians." ID215 |
| | Copyright & Training Data | Consent and transparency issues in training or generation. | "is built upon data without the consent of the artists that have dedicated decades of their lives to the craft" ID615 |
| | Substitution of Artists | Assertions that AI will replace human composers/performers. | "the danger I see is that it will take over the function of the human composer" ID951 |
| Cultural / Artistic implications | Oversaturation of content / Slop | Fear / criticism of low-quality AI output. | "due to the accessibility of it, we will see much more slop than actual creativity going forward." ID615 |
| | Collaboration / Co-Creativity | Remarks about human–AI co-creation possibilities. | "If it can be used as an aid to composition as electronic devices |

| | | | |
|---|---|---|---|
| | | | have been, then it might be very useful", ID951 |
| | Skills related to AI Music | Recognition that AI music-making requires skill and talent. | "I have found that using AI generated music is something that requires talent and i appreciate it when i come across it." ID913 |
| | Effects on artistic process | Description of shifts in workflows and practices | "I think AI music generation can help musicians to creatively think and mentally work on their craft while leaving the heavy lifting to AI" ID426 |
| | Effects on human creativity | Impact on people's creative drive, learning, abilities. | "I would worry about what it means for human creativity" ID53 |
| | Effects on music culture | Remarks about how AI impacts the music landscape | "I fear that humanity gets used to this and unlearns the art of music." ID67 |
| Innovation / Opportunities | Democratization of music production | Lowered entry barriers enabling novices/non-musicians to create. | "It can open the door for people like me who love music but are not talented in singing or playing instruments." ID610 |
| | New possibilities for artists | Potential for artists to gain inspiration, e.g. invention of new genres. | "likely will even provide options the artist may not have thought of to make the music even better" ID613 |
| | Curiosity | Neutral/curious interest in exploring AI tools. | "It can be great to hear what AI comes up with" ID450 |
| | Technological fascination | Wonder, impressive comments about the technical status quo | „It's fascinating that this works." (Original: "Es ist faszinierend, dass dies funktioniert."), ID85 |
| Functional Use / Contextual Value | Usefulness / Functional music | Background/ambient use cases (study, relaxation, therapy, commercial). | "it's used for a kind of purpose where music is not exactly the focus. So Ai generated background music is completely fine", ID946 |
| | Personalization | Tailoring music to individual preferences or moods | "AI-generated music could provide more personalized music for your tastes.", ID55 |
| | Productivity / Optimization | Remarks about efficiency/workflow gains. | "instead of the artist spending months to create the "perfect" music, AI will allow them to create in much less time", ID613 |
